# Supplementary material for: A minimal statistical-mechanical model for multihyperuniform patterns in avian retina
Source: arXiv:2005.01558 source file (2020-05-04)
Supplement: Supplementary file 1 [file retina-SI.pdf]

# A minimal statistical-mechanical model for multihyperuniform patterns in avian retina. Supplementary Information

Enrique Lomba[1], Jean-Jacques Weis[3], Leandro Guisández[1,2], and Salvatore Torquato[4,5]
[1]*Instituto de Química Física Rocasolano, CSIC, Calle Serrano 119, E-28006 Madrid, Spain*
[2]*IFLYSIB (UNLP, CONICET), 59 No. 789, B1900BTE La Plata, Argentina*
[3]*Université de Paris-Sud, Laboratoire de Physique Théorique, UMR8627, Bâtiment 210, 91405 Orsay Cedex, France*
[4]*Department of Chemistry, Princeton University, Princeton, New Jersey 08544, USA*
[5]*Princeton Institute for the Science and Technology of Materials, Princeton University, Princeton, New Jersey 08544, USA*

## A. A general condition for multihyperuniformity in mixtures

In the general case of a $n$-component mixture, the Ornstein-Zernike equation in Fourier space reads

$$\tilde{h}_{ij}(Q) = \tilde{c}_{ij}(Q) + \sum_l \tilde{c}_{il}(Q)\rho_l \tilde{h}_{lj}(Q) \tag{S.1}$$

where $\tilde{h}_{ij}(Q)$ and $\tilde{c}_{ij}(Q)$ are the Fourier transforms of the total correlation function, $h_{ij}(r)$, and the direct correlation function, $c_{ij}(r)$ respectively, $\rho_l$ is the number density of species $l$, and the subscripts denote different species. This gives for the symmetrized partial structure factors

$$\delta_{ij} + (\rho_i\rho_j)^{1/2}\tilde{h}_{ij}(Q) = \frac{\mathbf{M}_{ij}(Q)}{|\mathbf{I}-\mathbf{C}|}. \tag{S.2}$$

Here $\mathbf{M}_{ij}$ is the $(ij)$ minor of the $\mathbf{I}-\mathbf{C}$ matrix, $\mathbf{I}$ is the identity matrix, $[\mathbf{C}]_{ij} = (\rho_i\rho_j)^{1/2}\tilde{c}_{ij}(Q)$ and $|\ldots|$ denotes the determinant of the $n \times n$ matrix. When this quantity vanishes as $Q \to 0$, the system will be multi-hyperuniform.

Now, if

$$\lim_{Q\to 0} \tilde{c}_{ii}(Q) \propto Q^{-\alpha} \;\; \forall\, i, \tag{S.3}$$

with $\alpha > 0$, then

$$\lim_{Q\to 0} M_{ij}(Q) \propto Q^{-(n-1)\alpha} \tag{S.4}$$

Additionally, one might expand the denominator in (S.2) [1]

$$|\mathbf{I}-\mathbf{C}| = 1 - |\mathbf{C}| - \sum_{i=1}^{n-1} \Gamma_n^i |\mathbf{C}/\mathbf{I}^i| \tag{S.5}$$

where $\Gamma_n^i|\mathbf{C}/\mathbf{I}^i|$ is the sum of the combination of determinants in which the $i$-th row of $\mathbf{C}$ is replaced by the corresponding row of $\mathbf{I}$. Now, when $|\mathbf{C}| \neq 0$, it turns out that

$$\lim_{Q\to 0} |\mathbf{I}-\mathbf{C}| = -\lim_{Q\to 0} |\mathbf{C}| \propto Q^{-n\alpha}. \tag{S.6}$$

It can be shown that

$$|\mathbf{C}| = (\prod_{i=1}^{m} \rho_i)|\mathbf{c}| \tag{S.7}$$

with $[\mathbf{c}]_{ij} = \tilde{c}_{ij}(Q)$. When Eq.(S.3) is satisfied, then $\lim_{Q\to 0} \tilde{c}_{ij}(Q) = -\lim_{Q\to 0} \beta\tilde{u}_{ij}(Q)$, by which, $\lim_{Q\to} \beta\tilde{u}_{ij}(Q) \propto Q^{-\alpha}$, using Eqs.(S.4), (S.6), and (S.2) one gets

$$\lim_{Q\to 0} \left(\delta_{ij} + (\rho_i\rho_j)^{1/2}\tilde{h}_{ij}(Q)\right) \propto Q^{\alpha} \;\; \forall\, (i,j), \tag{S.8}$$

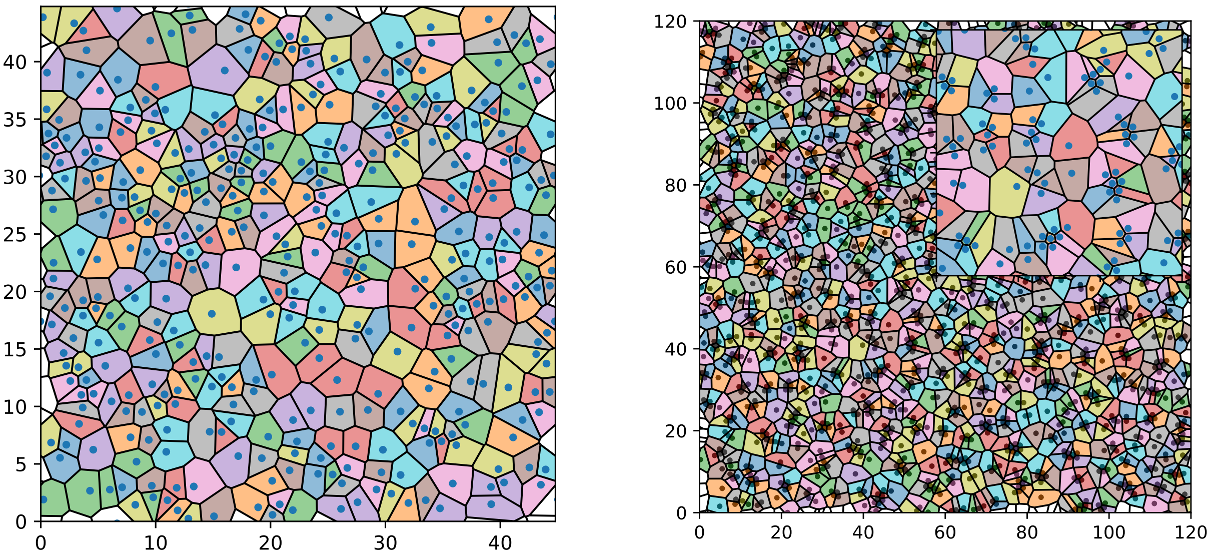


(a)LJ, $\rho\sigma^2 = 0.2$

(b)LJ, $\rho\sigma^2 = 0.8$

FIG. 1. Voronoi tessellations corresponding to a LJ fluid configuration for $\rho\sigma^2 = 0.2$ (left) and a LJ fluid with added Coulomb repulsion at $\rho\sigma^2 = 0.1111$, and $k_BT/\epsilon = 2$ (right). The inset on the right figure is a zoom of the central area of the simulation cell. Effects of clustering due to the competing short range attraction and long range repulsion are clearly seen. The low density LJ configuration yields a Voronoi tessellation indistinguishable from that of a random configuration of points.

and therefore all the structure factors will vanish as $Q \to 0$. This implies that the system will be multi-hyperuniform, if the conditions

$$\lim_{Q\to 0} \beta \tilde{u}_{ii}(Q) \propto Q^{-\alpha} \tag{S.9}$$

$$\lim_{Q\to 0} |\tilde{\mathbf{u}}(Q)| \neq 0 \tag{S.10}$$

are satisfied, where $[\mathbf{u}]_{ij} = \tilde{u}_{ij}(Q)$. This is a generalization of Eq. (7) in Ref. [2].

### B. Asymptotics in the symmetric three-component case.

In the case of mixtures one must monitor the small wavenumber behavior the partial structure factors. These quantities can be expressed in terms of the corresponding atom-atom total correlation functions as

$$S_{ij}(Q) = x_i \left( \delta_{ij} + \rho x_j \tilde{h}_{ij}(Q) \right). \tag{S.11}$$

Now, when all densities are identical, such that $\rho_i = \rho/3\ \forall i$, being $\rho$ the total number density, and the interactions are given by Eq. (5), one can solve Eq. (S.1) in Fourier space and obtain for the partial structure factors

$$\begin{aligned} \lim_{Q\to 0} S_{ii}(Q) &= Q^2 \frac{Q^2 - \rho_1(\tilde{c}^R_{11} + \tilde{c}^R_{12})Q^2 + 2\pi\rho_1\Gamma(1+\lambda)}{Q^4 \mathrm{det}|\mathbf{I} - \mathbf{C}|} \\ \lim_{Q\to 0} S_{ij}(Q) &= x_i \left( \delta_{ij} + \rho x_j Q^2 \frac{\tilde{c}^R_{ij} Q^2 - 2\pi\rho_i \Gamma\lambda}{Q^4 \mathrm{det}|\mathbf{I} - \mathbf{C}|} \right) \end{aligned} \tag{S.12}$$

with $i \neq j$, and with the determinant in the denominator given by

$$\begin{aligned} Q^4 \mathrm{det}|\mathbf{I} - \mathbf{C}| = &(Q^2 - \rho_i(\tilde{c}^R_{ii} - \tilde{c}^R_{ij})Q^2 + 2\pi\rho_1\Gamma(1-\lambda)) \\ &\times (Q^2 - \rho_1(\tilde{c}^R_{ii} + 2\tilde{c}^R_{ij})Q^2 + 2\pi\rho_i\Gamma(1+2\lambda))) \end{aligned}$$

where the Fourier transforms of the direct correlation functions are separated into a short range component ($\tilde{c}^R_{ii}(Q)$ and $\tilde{c}^R_{12}(Q)$) and Coulomb like contributions, namely, $\tilde{c}_{ii}(Q) = \tilde{c}^R_{ii}(Q) + 2\pi\Gamma/Q^2$, $\forall i$, and $\tilde{c}_{ij} = \tilde{c}^R_{ij}(Q) + 2\pi\lambda\Gamma/Q^2$, $\forall i \neq j$. We know that the zero wavenumber limit of the short range components is always finite and non-zero.

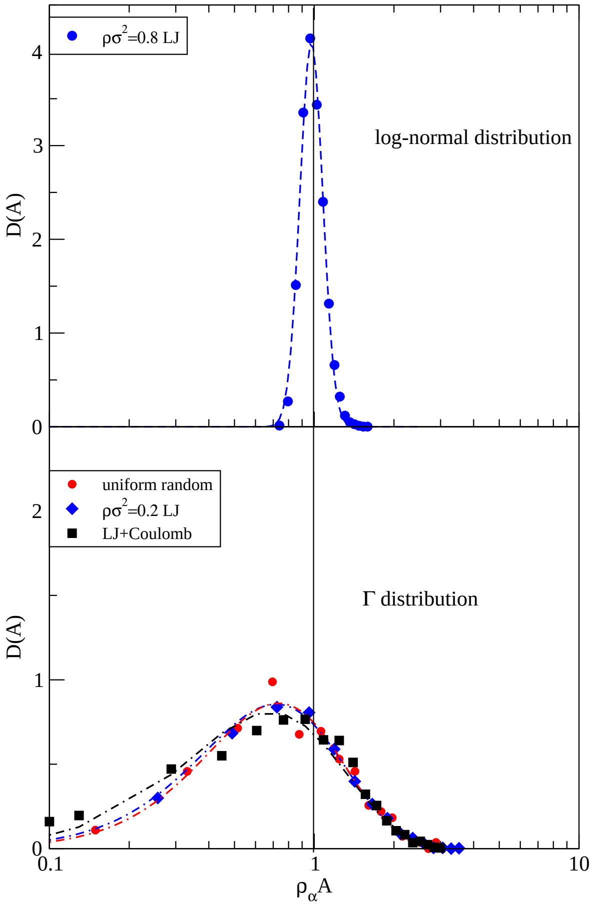


FIG. 2. Scaled area distribution of the Voronoi polygons for LJ+repulsive Coulomb and LJ interacting particles together with random configurations. Dashed lines correspond to fits to Eqs. (S.13) and (S.14). The random and low density LJ configurations (lower graph) agree with Γ-distributions – Eqs. (S.13–, whereas when correlation effects become appreciable (upper graph) the curves follow an apparent log-normal distribution –Eq. (S.14)–. Notice the log scale on the $\rho A$ axis.

From Eq. (S.12) we find that whenever $\lambda \neq 1$ and $\lambda \neq -1/2$ then $\lim_{Q\to 0} S_{ii}(Q) \propto Q^2$, for all species, that is, the system will be multi-hyperuniform. Also, in the fully symmetric case, $\lambda = -1/2$ corresponds precisely to a two-dimensional Coulomb electrolyte, where we have 1/3 of the particles with charge +1 and 2/3 of the particles with charge -1/2. This system will then behave as a "regular fluid" and does not even display global hyperuniformity due to the screening effects [2]. The $\lambda = 1$ case will not be multi-hyperuniform, but will preserve the global hyperuniformity of the single component two dimensional Coulomb plasma.

### C. Voronoi analysis

In order to put these results for our photoreceptor model in perspective, we have also performed a corresponding analysis for purely random two dimensional point configurations, as well as configurations obtained from Molecular Dynamics simulations for 2D fluids of Lennard-Jones (LJ) particles, and a LJ fluid with an additional long range repulsive Coulomb interaction. For these we have used similar density conditions and supercritical temperatures ($k_B T/\epsilon = 2.0$, where $k_B$ is Boltzmann's constant and $T$ the absolute temperature). When referring to LJ results, $\epsilon$ and $\sigma$ correspond to the well depth and particle size respectively. In Figure 1 and one can clearly appreciate that the

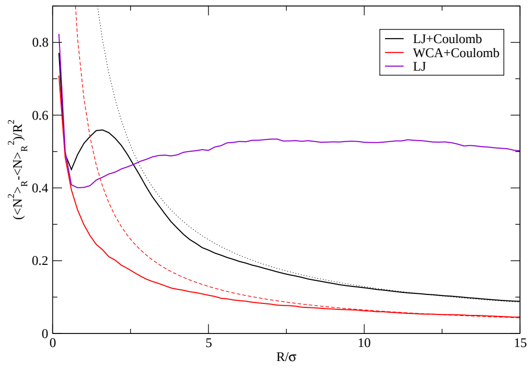


FIG. 3. Scaled number variance $\sigma_N^2(R)/R^2$ dependence of sample window radius, $R$, for LJ, LJ+Coulombic repulsion, and purely repulsive soft potential (LJ cut and shifted at $r/\sigma = 2^{1/6}$,i.e. WCA)+Coulombic repulsion. The last two systems are hyperuniform and hence $\sigma_N^2(R)/R^2 \to 0$. Due to the the presence of clustering, LJ+Coulomb repulsion exhibit a clear non-monotonous behavior for $R/\sigma < 4$.

areas of the Voronoi polygons are rather different in size, which is in contrast with the results seen for our model with pure long-range logarithmic repulsion. This can be more quantitatively analyzed taking a look at the normalized area distributions. These are plotted in Figure 2 vs the area scaled with the corresponding particle densities, $\rho A$.

The area distribution of Voronoi polygons from random point configurations is known to follow approximately a $\Gamma$ distribution of the form[3]

$$pdf(x) = \frac{c}{\Gamma(c)} x^{c-1} e^{-cx} \tag{S.13}$$

where $c$ is a fitting parameter and $\Gamma(c)$ is the transcendental $\Gamma$-function. In Figure 2 one can see that the distributions for low density LJ and purely random point configurations can accurately be fitted to Eq. (S.13). In the upper graph of Figure 2 we have results for the single species configuration for the LJ fluid at $\rho\sigma^2 = 0.8$. In this instance correlations are important and no reasonable fit to Eq. (S.13) is possible. Interestingly, the curves apparently follow a log-normal distribution, an ubiquitous distribution that describes multiple natural growth processes due to accumulation. The corresponding functional form is

$$pdf(x) = \frac{1}{\sqrt{2\pi\varsigma^2 x^2}} \exp\left(-\log(x/\mu)^2/(2\varsigma^2)\right) \tag{S.14}$$

where $\varsigma$ and $\mu$ are two fitting parameters. Note that the curve is plotted vs. $\rho A$ in a log-scale and looks almost Gaussian. This should be exactly the case when the distribution follows Eq. (S.14). The vertical line represents the $\delta$ function distribution corresponding to the Voronoi tessellation of the regular square lattice, i.e. $\delta(\rho A - 1)$ and one can see that the curves are not symmetric with respect to it.

Finally, in figure 3 we illustrate the sampling window dependence of the scaled number variance

$$\sigma_N^2(R) = \left(\langle N^2\rangle_R - \langle N\rangle_R^2\right)/R^2$$

for two disordered hyperuniform systems, one composed of LJ particles with added Coulombic repulsion (which exhibits stable clusters), and the other with cut and shifted LJ interactions at $2^{1/6}\sigma$, plus Coulombic repulsion, compared with a plain LJ system (non-hyperuniform). The number variance in the latter instance is monotonous and scales quadratically with, $R$, whereas the for both hyperuniform system it scales linearly, and in the presence of clustering a marked non-monotonous behavior is apparent for small sampling windows.

[1] S. J. Xu, M. Darouach, and J. Schaefers, IEEE Trans. Automat. Contr. **38**, 1671 (1993).
[2] E. Lomba, J.-J. Weis, and S. Torquato, Phys. Rev. E **97**, 010102(R) (2018).
[3] M. Ferraro and L. Zaninetti, Physica A: Statistical Mechanics and its Applications **391**, 4575 (2012).
